# Supplementary material for: ChatBI: Towards Natural Language to Complex Business Intelligence SQL
Source: arXiv:2405.00527 source file (2024-05-01)
Supplement: Supplementary file 1 [file 7.appendix.tex]

\appendix

\section{Complex BI SQL Corresponding to Figure~\ref{figure:BIExample}}\label{appendix:executionSql}
\begin{lstlisting}[ language=SQL,
                    deletekeywords={IDENTITY},
                    deletekeywords={[2]INT},
                    morekeywords={clustered},
                    framesep=8pt,
                    xleftmargin=40pt,
                    framexleftmargin=25pt,
                    frame=tb,
                    framerule=0pt ]
SELECT table_1Week_l.`xc_1` AS `xc_1`,
       table_1Week_l.`xc_2` AS `xc_2`,
       table_1Week_l.`mt_3` AS `mt_3`,
       (table_1Week_l.`mt_3` - table_1Week_l.
   `mt_4`) / table_1Week_l.`mt_4` AS `mt_4`,
       (table_1Week_l.`mt_3` - table_1Day.
   `mt_3`) / table_1Day.`mt_3` AS `mt_5`
FROM
  (SELECT table_origin.`xc_1` AS `xc_1`,
          table_origin.`xc_2` AS `xc_2`,
          table_origin.`mt_3` AS `mt_3`,
          table_origin.`a` AS `a`,
          table_1Week.`mt_3` AS `mt_4`
   FROM
     (SELECT toDate(toDate(event_day)) AS 
     `xc_1`,
             city AS `xc_2`,
             sum(share_icon_cnt) AS `mt_3`,
             1 AS a
      FROM `test`.`chatbi_demo_dataset`
      WHERE toDate(event_day) >= '2024-01-19'
        AND toDate(event_day) <= '2024-01-25'
        AND city IN (`Beijing`, `Tianjin`)
      GROUP BY xc_1,
               xc_2) AS `table_origin`
   LEFT OUTER JOIN
     (SELECT toDate(dateAdd(WEEK, 1, toDate(
     toDate(event_day)))) AS `xc_1`,
             city AS `xc_2`,
             sum(share_icon_cnt) AS `mt_3`
      FROM `test`.`chatbi_demo_dataset`
      WHERE toDate(event_day) >= '2024-01-12'
        AND toDate(event_day) <= '2024-01-18'
        AND city IN (`Beijing`, `Tianjin`)
      GROUP BY xc_1,
               xc_2) AS `table_1Week` ON 
      table_origin.`xc_1` = table_1Week.`xc_1`
   AND table_origin.`xc_2` = table_1Week.
       `xc_2`) AS `table_1Week_l`
LEFT OUTER JOIN
  (SELECT toDate(dateAdd(DAY, 1, toDate(
  toDate(event_day)))) AS `xc_1`,
          city AS `xc_2`,
          sum(share_icon_cnt) AS `mt_3`
   FROM `test`.`chatbi_demo_dataset`
   WHERE toDate(event_day) >= '2024-01-18'
     AND toDate(event_day) <= '2024-01-24'
     AND city IN (`Beijing`, `Tianjin`)
   GROUP BY xc_1,
            xc_2) AS `table_1Day` ON 
      table_1Week_l.`xc_1` = table_1Day.`xc_1`
AND table_1Week_l.`xc_2` = table_1Day.`xc_2`
ORDER BY `xc_1` ASC,
         `mt_3` DESC
LIMIT 10000
\end{lstlisting}
Here, "xc" represents a column, "mt" represents a metric, and the field names have been desensitized.
